# Supplementary material for: OpenRL: A Unified Reinforcement Learning Framework
Source: arXiv:2312.16189 source file (2023-12-20)
Supplement: Supplementary file 1 [file appendix_lib_compare.tex]

\section{Comparison of OpenRL to existing popular RL libraries. }
\label{ap:lib_compare}
\input{tables/lib_compare}
